# Supplementary material for: Engineering the Floquet spectrum of superconducting multiterminal quantum dots
Source: arXiv:1903.04889 ancillary file (2019-08-02)
Supplement: Supplementary file 1 [file supplemental-material5-revised.pdf]

# Floquet spectrum and finite frequency noise in multiterminal quantum dot Josephson junctions: Supplemental Material


Régis Mélin,[1] Romain Danneau,[2] Kang Yang,[3,4] Jean-Guy Caputo,[5] and Benoît Douçot[3]

[1] *Univ. Grenoble-Alpes, CNRS, Grenoble INP, Institut NEEL, 38000 Grenoble, France*

[2] *Institute of Nanotechnology, Karlsruhe Institute of Technology, D-76021 Karlsruhe, Germany*

[3] *Laboratoire de Physique Théorique et Hautes Energies, Sorbonne Université and CNRS UMR 7589, 4 place Jussieu, 75252 Paris Cedex 05, France*

[4] *Laboratoire de Physique des Solides, CNRS UMR 8502, Univ. Paris-Sud, Université Paris-Saclay F-91405 Orsay Cedex, France*

[5] *Laboratoire de Mathématiques, INSA de Rouen, Avenue de l'Université, F-76801 Saint-Etienne du Rouvray, France*



(Dated: August 2, 2019)


The Supplemental Material provides the necessary details on the sharp resonance approximation: i) the demonstration of Eq. (7) (in the paper) for the resolvent in section IV A of the paper, and ii) that of Eqs. (9)-(11) for the charge-charge correlation function in section IV B. The general framework of Bogoliubov-de Gennes (BdG) equations is introduced in the following section I for the device shown in Fig. 1 of the paper. Section II presents a demonstration of this Eq. (7) (in the paper), which is injected into the expression of the local dot propagator. The calculation is next generalized in section III and IV to the dc-charge density and the dc-currents respectively. Appendix A provides further details on the form of the resolvent in the sharp resonance approximation. Appendix B details the spectral decomposition of the currents.

## I. FLOQUET QUASIPARTICLE BASIS

The Hamiltonian $\mathscr{H}$ is provided in Eqs. (20)-(21) of the Appendix (in the paper). Because it is quadratic in the basic fermion operators, a complete solution is obtained from the solution of the time-dependent Bogoliubov-de Gennes (BdG) equation

$$i\frac{d}{dt}\Gamma^\dagger(t) = [\mathscr{H}(t), \Gamma^\dagger(t)], \tag{1}$$

where $\Gamma^\dagger(t)$ denotes the quasi-particle creation operator. The Hamiltonian being periodic in time $t$ (with period $T = 2\pi/\omega_0$, where $\omega_0 = eV/\hbar$ in the presence of finite bias voltage $V$), we follow the Floquet prescription to impose the periodicity conditions $\Gamma^\dagger(t+T) = \exp(-iET/\hbar)\Gamma^\dagger(t)$. We note that taking the hermitian conjugate of Eq. (1) generates another Floquet solution $\Gamma(t)$, with $E$ changed into its opposite.

The quasi-particle spectrum has mixed nature in equilibrium (*i.e.* when $V$ is vanishingly small). It is composed of: i) a continuum of quasiparticles $\gamma^\dagger_\sigma(j,\mathbf{k})$, with corresponding energies $E(j,\mathbf{k}) = \sqrt{\varepsilon(j,\mathbf{k})^2 + |\Delta_j|^2}$, and ii) an $SU(2)$ spin doublet of Andreev bound-states (ABS) at positive energy below $|\Delta_j|$ for all $j$. We use here the convention that quasiparticle creation operators are associated to positive energies, while the corresponding destruction operators have the opposite (hence negative) energy. As emphasized in the Introduction of the paper, ABS are replaced by Floquet-Wannier-Stark (FWS) ladders of resonances at finite bias voltage. In the Floquet basis, we have then only continuous spectrum of dressed quasiparticle states in the entire energy range. Basic ideas from scattering theory are now used to compute these states explicitely.

Let us assume that the bare quasi-particle operator $\gamma^\dagger_\sigma(j,\mathbf{k})$ evolves into the dressed operator $\Gamma^\dagger_\sigma(j,\mathbf{k})$ as the tunneling terms $J_j$ are switched on adiabatically. Taking into account $SU(2)$ spin symmetry leads to the following expansion

$$\Gamma^\dagger_\sigma(j,\mathbf{k};t) = e^{-iE(j,\mathbf{k})t/\hbar}\gamma^\dagger_\sigma(j,\mathbf{k}) + e^{-iE(j,\mathbf{k})t/\hbar}\sum_{m\in\mathbb{Z}} e^{-im\omega_0 t}(u_m(j,\mathbf{k})d^\dagger_\sigma + \sigma v_m(j,\mathbf{k})d_{-\sigma})$$
$$+ e^{-iE(j,\mathbf{k})t/\hbar}\sum_{m\in\mathbb{Z}} e^{-im\omega_0 t}\sum_{i=1}^{N}\int\frac{d^D\mathbf{k}'}{(2\pi)^D}\left(u_m(i,\mathbf{k}';j,\mathbf{k})c^\dagger_\sigma(i,\mathbf{k}') + \sigma v_m(i,\mathbf{k}';j,\mathbf{k})c_{-\sigma}(i,\mathbf{k}')\right). \tag{2}$$

With this Ansatz, and introducing an infinitesimal positive damping rate $\eta$, the general BdG equation turns into the Lippmann-Schwinger equation for dressed Floquet operators

$$(E(j,\mathbf{k})+m\omega_0-\varepsilon(i,\mathbf{k}')+i\eta)u_m(i,\mathbf{k}';j,\mathbf{k}) = \Delta_i v_m(i,\mathbf{k}';j,\mathbf{k})+J_i u_{m-s_i}(j,\mathbf{k}) \tag{3}$$

$$(E(j,\mathbf{k})+m\omega_0+\varepsilon(i,\mathbf{k}')+i\eta)v_m(i,\mathbf{k}';j,\mathbf{k}) = \Delta_i^* u_m(i,\mathbf{k}';j,\mathbf{k})-J_i v_{m+s_i}(j,\mathbf{k}), \tag{4}$$

and

$$(E(j,\mathbf{k})+m\omega_0+i\eta)u_m(j,\mathbf{k}) = J_i\int\frac{d^D\mathbf{k}'}{(2\pi)^D}u_{m+s_i}(i,\mathbf{k}';j,\mathbf{k})+J_j\delta_{m,-s_j}x(j,\mathbf{k})e^{i\varphi_j/2} \tag{5}$$

$$(E(j,\mathbf{k})+m\omega_0+i\eta)v_m(j,\mathbf{k}) = -J_i\int\frac{d^D\mathbf{k}'}{(2\pi)^D}v_{m-s_i}(i,\mathbf{k}';j,\mathbf{k})-J_j\delta_{m,s_j}y(j,\mathbf{k})e^{-i\varphi_j/2}. \tag{6}$$

Here, we have set $\Delta_j = e^{i\varphi_j}|\Delta_j|$. The bare quasiparticle creation operators in the reservoirs are given by $\gamma_\sigma^\dagger(j,\mathbf{k}) = x(j,\mathbf{k})e^{i\varphi_j/2}c_\sigma^\dagger(j,\mathbf{k})+\sigma y(j,\mathbf{k})e^{-i\varphi_j/2}c_{-\sigma}(j,-\mathbf{k})$, with

$$x(j,\mathbf{k}) = \sqrt{\frac{1}{2}\left(1+\frac{\varepsilon(j,\mathbf{k})}{E(j,\mathbf{k})}\right)} \text{ and } y(j,\mathbf{k}) = \sqrt{\frac{1}{2}\left(1-\frac{\varepsilon(j,\mathbf{k})}{E(j,\mathbf{k})}\right)}. \tag{7}$$

Using Eqs. (3), (4) to eliminate amplitudes in the reservoirs, and substituting into Eqs. (5), (6) leads to

$$(E+m\omega_0+i\eta)u_m(j,\mathbf{k})-\sum_{i=1}^{N}J_i^2\,U_m^{(i)}(j,\mathbf{k}) = J_j\delta_{m,-s_j}x(j,\mathbf{k})e^{i\varphi_j/2} \tag{8}$$

$$(E+m\omega_0+i\eta)v_m(j,\mathbf{k})-\sum_{i=1}^{N}J_i^2\,V_m^{(i)}(j,\mathbf{k}) = -J_j\delta_{m,s_j}y(j,\mathbf{k})e^{-i\varphi_j/2}, \tag{9}$$

where

$$U_m^{(i)}(j,\mathbf{k}) = g_{11}^{(i)}(E+(m+s_i)\omega_0)u_m(j,\mathbf{k})-g_{12}^{(i)}(E+(m+s_i)\omega_0)v_{m+2s_i}(j,\mathbf{k}) \tag{10}$$

$$V_m^{(i)}(j,\mathbf{k}) = -g_{21}^{(i)}(E+(m-s_i)\omega_0)u_{m-2s_i}(j,\mathbf{k})+g_{22}^{(i)}(E+(m-s_i)\omega_0)v_m(j,\mathbf{k}). \tag{11}$$

Here, we used the short notation $E\equiv E(j,\mathbf{k})$. In a forthcoming paper on semi-classical theory, we will make extensive use of the linear operator $\mathscr{L}(E)$ acting on the collection of amplitudes $u_m(j,\mathbf{k})$, $v_m(j,\mathbf{k})$ [see the left-hand-side of Eqs. (8) and (9).] The function $g_{ab}^{(i)}(\omega)$ is the Fourier transform of the retarded Green's function $g_{\mathrm{ret}}^{(i)}(t)$ of the isolated reservoir $i$ on the tunneling site connected to the dot, defined as

$$g_{\mathrm{ret}}^{(i)}(t) = -i\begin{pmatrix} \{\Psi_{i,\sigma}(t),\Psi_{i,\sigma}^\dagger(0)\} & \sigma\{\Psi_{i,\sigma}(t),\Psi_{i,-\sigma}(0)\} \\ \sigma\{\Psi_{i,-\sigma}^\dagger(t),\Psi_{i,\sigma}^\dagger(0)\} & \{\Psi_{i,-\sigma}^\dagger(t),\Psi_{i,-\sigma}(0)\}\end{pmatrix}$$

for $t>0$ and $g_{\mathrm{ret}}^{(i)}(t)=0$ for $t<0$. Here $\Psi_{i\sigma}=\int\frac{d^D\mathbf{k}'}{(2\pi)^D}c_\sigma(i,\mathbf{k}')$. Explicitely, assuming that $\Im\omega>0$, we have

$$g^{(i)}(\omega) = \int\frac{d^D\mathbf{k}'}{(2\pi)^D\mathscr{D}(\omega,i,\mathbf{k}')}\begin{pmatrix}\omega+\varepsilon(i,\mathbf{k}') & \Delta_i \\ \Delta_i^* & \omega-\varepsilon(i,\mathbf{k}')\end{pmatrix},$$

where $\mathscr{D}(\omega,i,\mathbf{k}')=\omega^2-E(i,\mathbf{k}')^2$. An important property of $\mathscr{L}(E)$ is its invariance under simultaneous translations of $m$ and $E$. If $\mathscr{T}$ is the operator which sends $m$ into $m+1$, we have

$$\mathscr{L}(E+p\omega_0) = \mathscr{T}^{-p}\mathscr{L}(E)\mathscr{T}^p, \tag{12}$$

or, equivalently:

$$\mathscr{L}(E+p\omega_0)_{m,n} = \mathscr{L}(E)_{m+p,n+p}. \tag{13}$$

Here, we have dropped Nambu indices to simplify the notation.

Denoting by $\mathscr{R}(E)$ the inverse of $\mathscr{L}(E)$, we can therefore express amplitudes on the dot by

$$w_m(j,\mathbf{k}) = J_j\mathscr{R}(E)_{m,w;-s_j,u}\,x(j,\mathbf{k})e^{i\varphi_j/2} - J_j\mathscr{R}(E)_{m,w;s_j,v}\,y(j,\mathbf{k})e^{-i\varphi_j/2}. \tag{14}$$

Here $w$ stands for either $u$ or $v$. Using unitarity of time evolution, it is then easy to express Heisenberg operators on the dot in terms of the dressed quasiparticle operators. Writing $\Gamma_\sigma^\dagger(j,\mathbf{k};t=0)=\Gamma_\sigma^\dagger(j,\mathbf{k})$, we get

$$d_\sigma^\dagger(t) = \sum_{j=1}^{N}\int\frac{d^D\mathbf{k}}{(2\pi)^D}\sum_{m\in\mathbb{Z}}e^{i(E(j,\mathbf{k})+m\omega_0)t}u_m^*(j,\mathbf{k})\Gamma_\sigma^\dagger(j,\mathbf{k})-\sigma e^{-i(E(j,\mathbf{k})+m\omega_0)t}v_m(j,\mathbf{k})\Gamma_{-\sigma}(j,\mathbf{k}). \tag{15}$$

Eqs. (14 and (15) give the possibility to evaluate correlation functions of an arbitrary number of local dot operators in the stationary state $|S\rangle$. Indeed, to define $|S\rangle$, we simply require that it satisfies $\Gamma_\sigma(j,\mathbf{k})|S\rangle = 0$ for any $(j,\mathbf{k})$ and $\sigma$. This prescription is equivalent to the usual Keldysh procedure, because the above dressed quasiparticle operators are obtained from the bare ones by an adiabatic switching process. We note that spectral decompositions analogous to Eq. (15) can also be written for the Heisenberg operators $\Psi^\dagger_{i\sigma}(t)$ on the reservoir sites coupled to the dot. The corresponding expressions are given in the following Appendix B. They are used to study various correlation functions: i) the dot propagator in section II below; ii) the charge-charge correlation function on the dot discussed in section III below and in sections IV A and IV B in the paper; iii) the dc-currents in the forthcoming section IV).

## II. LOCAL DOT PROPAGATORS

Since the Hamiltonian is quadratic in fermion operators at all times, all correlations functions of physical observables in the stationary state $|S\rangle$ obey Wick's theorem, so their computation reduces to the evaluation of expectation values of fermionic bilinears. As a first example, let us consider

$$\langle S|d_\sigma(t)d^\dagger_\sigma(t')|S\rangle = \sum_{j=1}^{N}\int \frac{d^D\mathbf{k}}{(2\pi)^D}\sum_{(m,m')\in\mathbb{Z}^2} e^{-i(E(j,\mathbf{k})+m\omega_0)t}e^{i(E(j,\mathbf{k})+m'\omega_0)t'}u_m(j,\mathbf{k})u^*_{m'}(j,\mathbf{k}). \quad (16)$$

In order to go further, we will need several properties of the resolvent $\mathscr{R}(E)$ [see Eq. (6) in the paper]. It will be discussed in a forthcoming paper that $|u_m(j,\mathbf{k})|$ contributes mostly when $(m, E = E(j,\mathbf{k}))$ belongs to a classically allowed region, *i.e.* when $E+m\omega_0$ lies inside one of the two energy intervals corresponding to the Andreev level bands.

When this condition is satisfied, we also expect that, for small voltages compared to superconducting gaps $|\Delta_j|$, the energy dependence of these amplitudes is sharply peaked around the centers of Wannier-Stark resonances at $E = E_\alpha + p\omega_0$, $p$ integer, $|E_\alpha| \le \omega_0/2$, where $\alpha \in \{+,-\}$ labels Wannier-Stark ladders. This choice of labels is motivated by the fact that taking the hermitian conjugate of a Floquet solution of the BdG equation with quasi-energy $E$ gives another solution with quasi-energy $-E$. From this, we deduce that $E_+ + E_- \equiv 0$ mod $\omega_0$.

In the limit of sharp resonances, it is natural to expect that the $\mathbf{k}$ integration will be well approximated by a discrete sum over $\alpha$ and $p$. At this point, it is convenient to use the covariance of the resolvent under translations deriving from Eq. (13):

$$\mathscr{R}(\tilde{E}+p\omega_0)_{m,n} = \mathscr{R}(\tilde{E})_{m+p,n+p}. \quad (17)$$

As shown in Appendix A [see Eq. (A9)], this assumption of sharp resonances leads to the following approximation for the resolvent: $\mathscr{R}(E)$:

$$\mathscr{R}(\tilde{E}+p\omega_0)_{m,n} \simeq \sum_{\alpha=\pm}\frac{\Psi_{m+p}(E_\alpha)\otimes\Phi_{n+p}(E_\alpha)}{\tilde{E}-E_\alpha+i\Gamma_\alpha}, \quad (18)$$

which coincides with Eq. (7) in the paper. Here $\{\Psi_m(E)\}_{m\in\mathbb{Z}}$ is a zero eigenvector of the $\mathscr{L}(E)$ operator, and $\{\Phi_n(E)\}_{n\in\mathbb{Z}}$ is a zero eigenvector of the transposed operator. For a given $m$, $\Psi_m(E)$ is a two-component column vector (in Nambu space), and for a given $n$, $\Phi_n(E)$ is a two-component row vector, so that $\Psi_m(E)\otimes\Phi_n(E)$ is a two by two matrix. In Eq. (14), $n = \pm s_j$, so $n \in \{0,-1,1\}$. On the other hand, $E = E(j,\mathbf{k}) > |\Delta_j|$ and $|u_m(j,\mathbf{k})|$ is negligible unless $E+m\omega_0$ lies inside one of the Andreev bands. This implies that $E+m\omega_0 < |\Delta_j| < E+n\omega_0$ and then $m<n$. The general discussion given in Appendix A shows that the following asymptotic conditions hold:

$$\lim_{m\to-\infty}\Psi_m(E_\alpha) = 0, \quad \lim_{n\to\infty}\Phi_n(E_\alpha) = 0. \quad (19)$$

Let us now return to Eq. (16). The $\mathbf{k}$ integral can be recast as a combination of an angular integral, which is trivial if we assume rotational symmetry in the $D$-dimensional reservoirs, and an integration over $k = |\mathbf{k}|$. We can trade the latter variable by the energy $E = E(j,\mathbf{k})$. In each interval $-\frac{\omega_0}{2}+p\omega_0 < E < \frac{\omega_0}{2}+p\omega_0$, the amplitudes $u_m(j,\mathbf{k})$ and $u^*_{m'}(j,\mathbf{k})$ are peaked in the vicinity of $E_\alpha + p\omega_0$, $\alpha\in\{+,-\}$. Assuming that resonances are narrow, *i.e.* that $\Gamma_\alpha$ is much smaller than any other characteristic energy scale in the problem, we can approximate the integral

$$\int_{-\omega_0/2}^{\omega_0/2}\frac{d\tilde{E}}{2\pi}\frac{e^{-i\tilde{E}(t-t')}}{(\tilde{E}-E_\alpha+i\Gamma_\alpha)(\tilde{E}-E_{\alpha'}-i\Gamma_{\alpha'})} \quad (20)$$

by the same integral taken on the whole real line, whose value reads

$$\frac{e^{-iE_\alpha(t-t')}e^{-\Gamma_\alpha(t-t')}\theta(t-t')+e^{-iE_{\alpha'}(t-t')}e^{-\Gamma_{\alpha'}(t'-t)}\theta(t'-t)}{\Gamma_\alpha+\Gamma_{\alpha'}+i(E_\alpha-E_{\alpha'})}. \quad (21)$$

A further simplification occurs when the two FWS ladders are well separated, *i.e.* when $\Gamma_\alpha \ll |E_1-E_2|$. Then, we can keep only the diagonal contribution, corresponding to $\alpha=\alpha'$.

In the process of converting the $k$ integral to an energy integral, we have to solve the equation in $k$:

$$E(j,k) \equiv \sqrt{\varepsilon(j,k)^2+|\Delta_j|^2} = E_\alpha + p\omega_0. \quad (22)$$

Because of the existence of a Fermi surface in the normal state in the reservoirs, $\varepsilon(j,k_{\mathrm{F},j}) = 0$, we have two solutions of (22), either $k > k_{\mathrm{F},j}$ or $k < k_{\mathrm{F},j}$. To account for this, we introduce the binary variable $\tau\in\{>,<\}$. Let us denote by $k(j,\alpha,p,\tau)$ the solutions of (22). We now define $v(j,\alpha,p,\tau)$ by

$$v(j,\alpha,p,\tau) = \left(\frac{dE(j,k)}{dk}(k=k(j,\alpha,p,\tau))\right)^{-1}. \quad (23)$$

Finally, changing $m+p$ into $m$, the sharp resonance approximation leads to

$$\langle S|d_\sigma(t)d^\dagger_\sigma(t')|S\rangle = \sum_{j=1}^{N}\sum_{\alpha=\pm} S_{j,\alpha} \sum_{(m,m')\in\mathbb{Z}^2}^{(j)} e^{-\Gamma_\alpha|t-t'|}e^{-iE_\alpha(t-t')}e^{-i\omega_0(mt-m't')}\Psi_{m,u}(E_\alpha)\Psi^*_{m',u}(E_\alpha), \tag{24}$$

with

$$S_{j,\alpha} = \frac{\mathscr{A}_D J_j^2}{2(2\pi)^{D-1}\Gamma_\alpha}\sum_{p\in\mathbb{Z}}\sum_{\tau} \nu(j,\alpha,p,\tau)(k(j,\alpha,p,\tau))^{D-1}\theta(E_\alpha+p\omega_0-|\Delta_j|) \tag{25}$$
$$|\Phi(E_\alpha)_{-s_j+p,u}e^{i\varphi_j/2}x(j,k(j,\alpha,p,\tau))-\Phi(E_\alpha)_{s_j+p,v}e^{-i\varphi_j/2}y(j,k(j,\alpha,p,\tau))|^2.$$

In this expression, $\mathscr{A}_D$ stands for the area of the unit sphere in a $D$-dimensional Euclidean space, so $\mathscr{A}_1 = 2$, $\mathscr{A}_2 = 2\pi$, $\mathscr{A}_3 = 4\pi$. Eq. (25) above coincides with Eq. (10) in the paper, with the difference that Eq. (25) appears here in the expression of the dot propagator instead of the charge-charge correlation function treated in sections IV A and IV B in the paper. Further comments on the structure of Eqs. (24) and (25) above can be found after Eqs. (9)-(11) in the paper.

For the applications to be discussed below and in section IV B of the paper, we need expressions similar to Eq. (24) for the expectation values of other fermionic bilinears. These all have the same structure, excepted for the form factors, which read

$$\langle S|d_\sigma(t)d^\dagger_\sigma(t')|S\rangle \to \Psi_{m,u}\Psi^*_{m',u} \tag{26}$$
$$\langle S|d^\dagger_\sigma(t)d_\sigma(t')|S\rangle \to \Psi_{m,v}\Psi^*_{m',v} \tag{27}$$
$$\langle S|d^\dagger_\sigma(t)d^\dagger_{-\sigma}(t')|S\rangle \to -\sigma\Psi_{m,v}\Psi^*_{m',u} \tag{28}$$
$$\langle S|d_\sigma(t)d_{-\sigma}(t')|S\rangle \to \sigma\Psi_{m,u}\Psi^*_{m',v}. \tag{29}$$

The charge density on the quantum dot and the dc-currents are treated now in the Secs. III and IV of this Supplementary Material within the sharp resonance approximation. The charge-charge correlation function is discussed in section IV B of the paper.

## III. CHARGE DENSITY ON THE DOT

Using the previous discussion, we get the following Fourier expansion:

$$\sum_\sigma \langle S|d^\dagger_\sigma(t)d_\sigma(t)|S\rangle = \sum_{p\in 2\mathbb{Z}} A_p e^{-ip\omega_0 t}, \tag{30}$$

with

$$A_p = 2\sum_{j=1}^{N}\sum_{\alpha=\pm} S_{j,\alpha}\sum_{m\in\mathbb{Z}}^{(j)} \Psi_{m,v}(E_\alpha)\Psi^*_{m-p,v}(E_\alpha). \tag{31}$$

Here, both $m$ and $m-p$ are requested to have the same parity as $s_j$, so $p$ is even. Besides the $S_{j,\alpha}$ coefficients, the Fourier amplitudes $A_p$ involve the overlap between the wave function $m \to \Psi_{m,v}(E_\alpha)$ and its translate by $p$ lattice spacings. So the number of significant Fourier harmonics $A_p$ contains some information on the width of the Andreev level bands. We also see that near an avoided crossing between the two Wannier-Stark ladders, there is a strong hybridization between the two Andreev bands, and this will approximately double the number of significant harmonics in this Fourier decomposition, by comparison to the generic non degenerate situation.

## IV. DC-CURRENTS

In a similar way, denoting by $\hat{I}_i$ the current operator from the dot to reservoir $i$, we have the Fourier series:

$$\sum_\sigma \langle S|\hat{I}_{i,H}(t)|S\rangle = \sum_{p\in 2\mathbb{Z}} B_{i,p}e^{-ip\omega_0 t}. \tag{32}$$

The Fourier coefficients are given in Appendix B, and the narrow resonance approximation Eq. (B7) is found to be similar to the previous Eq. (31). We note that charge conservation is satisfied:

$$\sum_{i=1}^{N} B_{i,p} = ip\omega_0 A_p. \tag{33}$$

### Appendix A: Resolvent for infinite discrete 1D problems

#### 1. General considerations

This material is elementary, we include it here to provide a self contained presentation supporting Eq. (7) in the paper [identical to Eq. (18) above in the Supplemental Material.]

We consider a linear operator $\mathscr{L}$, acting on an infinite-dimensional vector space represented by sequences $(\Psi_m)_{m\in\mathbb{Z}}$. Here each $\Psi_m$ is an $M$-dimensional column vector. In the case of physical interest discussed in this paper, $M = 2$ since $\Psi_m$ can be viewed as a two-component Nambu spinor. The explicit form of $\mathscr{L}$ is the following:

$$(\mathscr{L}\Psi)_m = A_m\Psi_m + B_{m+1}\Psi_{m+2} + C_{m-1}\Psi_{m-2}. \tag{A1}$$

Here, $A_m$, $B_{m+1}$, and $C_{m-1}$ are arbitrary $M$ times $M$ matrices with complex coefficients. The only request we make is that $B_{m+1}$ and $C_{m-1}$ be invertible for all $m$. As a result, the family of solutions of the homogeneous equation $\mathscr{L}\Psi = 0$ forms a complex vector space $V$ of dimension $2M$, because we can choose arbitrary initial conditions $(\Psi_0, \Psi_1)$, and iteratively construct $\Psi_m$ such that $(\mathscr{L}\Psi)_m = 0$ for all $m$. For

the operator $\mathscr{L}(E)$, when $\Im E \geq 0$, $V$ can be written as a direct sum $V = V^+ \oplus V^-$, where $V^+$ (resp. $V^-$) is the subspace of zero eigenvectors such that $\lim_{m\to\infty}\Psi_m = 0$ (resp. $\lim_{m\to-\infty}\Psi_m = 0$). We note that $\mathscr{L}$ acts by right multiplication on dual vectors $(\Phi_n)_{n\in\mathbb{Z}}$, where each $\Phi_n$ is an $M$-dimensional row vector. Explicitely:

$$(\Phi\mathscr{L})_n = \Phi_n A_n + \Phi_{n-2}B_{n-1} + \Phi_{n+2}C_{n+1}. \qquad \text{(A2)}$$

Likewise, the $2M$-dimensional vector space $W$ of solutions of $\Phi\mathscr{L} = 0$ is most often decomposable as $W = W^+ \oplus W^-$.

The main interest is the resolvent operator $\mathscr{R}$ which is defined by $\mathscr{L}\mathscr{R} = \mathscr{R}\mathscr{L} = \mathbf{1}$, where $\mathbf{1}$ denotes the identity operator. We may visualize $\mathscr{R}$ as a doubly infinite collection $\mathscr{R}_{mn}$ of $M$ times $M$ matrices, which satisfy

$$A_m\mathscr{R}_{mn} + B_{m+1}\mathscr{R}_{m+2,n} + C_{m-1}\mathscr{R}_{m-2,n} = \delta_{mn}\mathbf{1}_M$$
$$\mathscr{R}_{mn}A_n + \mathscr{R}_{m,n-2}B_{n-1} + \mathscr{R}_{m,n+2}C_{n+1} = \delta_{mn}\mathbf{1}_M.$$

Introducing basis solutions $\Psi_m^{\alpha\pm}$ $(1 \leq \alpha \leq M)$ in $V^\pm$ and $\Phi_n^{\beta\pm}$ $(1 \leq \beta \leq M)$ in $W^\pm$, we may express the resolvent as

$$\mathscr{R}_{mn} = \sum_{\alpha\beta} c^>_{\alpha\beta}\Psi_m^{\alpha+}\otimes\Phi_n^{\beta-} \quad (m \geq n) \qquad \text{(A3)}$$

$$\mathscr{R}_{mn} = \sum_{\alpha\beta} c^<_{\alpha\beta}\Psi_m^{\alpha-}\otimes\Phi_n^{\beta+} \quad (m \leq n). \qquad \text{(A4)}$$

The coefficients $c^>_{\alpha\beta}$ and $c^<_{\alpha\beta}$ can be determined from the knowledge of the Wronskiens between basis functions. To define the Wronskian in such situation, let us pick a pair $(\Phi,\Psi)$ of solutions of $\Phi\mathscr{L} = 0$ and $\mathscr{L}\Psi = 0$. If we multiply (A1)by $\Phi_m$ on the left and (A2)by $\Psi_n$ on the right, set $l = m = n$ and then subtract the results, we see that the quantity $\Phi_l B_{l+1}\Psi_{l+2} - \Phi_{l+2}C_{l+1}\Psi_l$ is independent of $l$. This constant value is denoted by $W(\Phi,\Psi)$. Clearly $W(\Phi,\Psi) = 0$ when both $\lim_{l\to\infty}\Phi_l = 0$ and $\lim_{l\to\infty}\Psi_l = 0$ or when both $\lim_{l\to-\infty}\Phi_l = 0$ and $\lim_{l\to-\infty}\Psi_l = 0$. Given the above basis, we define Wronskian matrices $W^{+-}_{\beta\alpha} = W(\Phi^{\beta+},\Psi^{\alpha-})$ and $W^{-+}_{\beta\alpha} = W(\Phi^{\beta-},\Psi^{\alpha+})$. It can be shown that, when $B_m$ and $C_m$ are invertible for all $m$ the Wronskian induces a non-degenerate pairing, so when the assumptions $V = V^+ \oplus V^-$ and $W = W^+ \oplus W^-$ are satisfied, both $W^{+-}$ and $W^{-+}$ are invertible. Then, easy direct calculations show that

$$c^> = (W^{-+})^{-1} \qquad \text{(A5)}$$
$$c^< = -(W^{+-})^{-1}. \qquad \text{(A6)}$$

These expressions can be written in a more suggestive way when $W^{+-}$ and $W^{-+}$ are diagonalizable. Introducing right eigenvectors $x^{i\pm}$ and left eigenvectors $y^{i\pm}$ for $1 \leq i \leq M$, we set

$$W^{+-}x^{i-} = \lambda^{i+-}x^{i-}$$
$$W^{-+}x^{i+} = \lambda^{i-+}x^{i+}$$
$$y^{i+}W^{+-} = \lambda^{i+-}y^{i+}$$
$$y^{i-}W^{-+} = \lambda^{i-+}y^{i-}.$$

This allows us to define $(\sigma = \pm)$

$$\tilde{\Psi}^{i\sigma} = \sum_{\alpha=1}^{M} x^{i\sigma}_\alpha \Psi^{\alpha\sigma} \in V^\sigma$$
$$\tilde{\Phi}^{i\sigma} = \sum_{\beta=1}^{M} y^{i\sigma}_\beta \Phi^{\beta\sigma} \in W^\sigma.$$

With these definitions, the resolvent reads

$$\mathscr{R}_{mn} = \sum_{i=1}^{M} \frac{\tilde{\Psi}_m^{i+}\otimes\tilde{\Phi}_n^{i-}}{\lambda^{i-+}} \quad (m \geq n) \qquad \text{(A7)}$$

$$\mathscr{R}_{mn} = -\sum_{i=1}^{M} \frac{\tilde{\Psi}_m^{i-}\otimes\tilde{\Phi}_n^{i+}}{\lambda^{i+-}} \quad (m \leq n). \qquad \text{(A8)}$$

Let us now introduce an external complex parameter $E$. A resonance in the resolvent $\mathscr{R}(E)$ occurs when an eigenvalue $\lambda^{i+-}$ (and also $\lambda^{i-+}$) goes to zero as $E \to E_{\text{res}}$. One way to achieve this is to have non-trivial intersections $\Psi^{\text{res}} \in V^+\cap V^-$ and $\Phi^{\text{res}} \in W^+\cap W^-$. Then $W(\Phi^{\text{res}},\Psi) = 0$ for all $\Psi \in V$ and $W(\Phi,\Psi^{\text{res}}) = 0$ for all $\Phi \in W$. So $\Psi^{\text{res}}$ is a zero right eigenvector for both $W^{+-}$ and $W^{-+}$ and likewise, $\Phi^{\text{res}}$ is a zero left eigenvector for both $W^{+-}$ and $W^{-+}$ Assuming that the associated eigenvalue vanishes linearly as a function of $E - E_{\text{res}}$, there is a normalization of $\Phi^{\text{res}}$ and $\Psi^{\text{res}}$ such that

$$\mathscr{R}(E)_{mn} \simeq \frac{\Psi_m^{\text{res}}\otimes\Phi_n^{\text{res}}}{E - E_{\text{res}}}. \qquad \text{(A9)}$$

as $E \to E_{\text{res}}$.

### 2. 1D operators arising from hermitian problems

In our problem, the effective 1D operator $\mathscr{L}(E)$ arises after tracing out the reservoirs while solving the Floquet-Lippmann-Schwinger equations for dressed quasiparticle operators. The effect of reservoirs is encoded in the $A_m$, $B_m$, $C_m$ matrices via $E$-dependent self energies which involve the retarded Green's functions in the isolated reservoirs. Because the underlying quantum dynamics arises from an hermitian Hamiltonian, the resolvent thus defined cannot have poles in the upper complex $E$ plane. Poles may arise only after we analytically continue $E$ from $\Im E > 0$ to $\Im E < 0$ across the real axis. Let us suppose that $E$ is real, and that $|E + m\omega_0| < |\Delta_j|$ for all $j$, $(1 \leq j \leq N$, $N$ being the number of superconducting reservoirs). Then, self energies are real, and in such an $m$ interval, the corresponding operator $\mathscr{L}_0(E)$ is hermitian, meaning that $A_m = A_m^\dagger$, $B_m = C_m^\dagger$. The semi-classical treatment discussed in a forthcoming paper will reveal that, if we neglect non hermitian terms arising when $|E + m\omega_0| > |\Delta_j|$, there are poles in $\mathscr{R}_0(E)$ for $E = E_\alpha + p\omega_0$, $p$ integer and $E_\alpha$ real. These originate from the Andreev bound-states, which give rise to Wannier-Stark ladders at finite voltage bias. We now argue that, when we replace the hermitian $\mathscr{L}_0(E)$ by the true $\mathscr{L}(E)$, these poles on the real axis will be pushed slightly below it. In the previous subsection, we have seen that the condition for resonance is simply that $V^+(E)\cap V^-(E) \neq \{0\}$.

The key remark is that this condition defines a complex codimension one subset of the complex $E$ plane. Indeed, we can pick bases in subspaces $V^+(E)$ and $V^-(E)$ which are locally analytic functions of $E$. The condition $V^+(E)\cap V^-(E)\neq\{0\}$ is simply given by the vanishing of a $2M$ by $2M$ determinant $\det(E)$ built from these basis vectors, so that $\det(E)$ is also locally analytic in $E$. In the semi-classical picture, the non hermitian character of $\mathscr{L}(E)$ is manifested by the presence of an additional reflected evanescent wave generated when $E+m\omega_0$ crosses an energy gap at $\pm|\Delta_j|$. Measured near the center of the gap, i.e. for $E+m\omega_0\simeq 0$, the effect of these reflected waves on $V^\pm(E)$ is exponentially small in the inverse voltage. Therefore $\det(E)$ for the non-hermitian $\mathscr{L}(E)$ problem differs from $\det_0(E)$ for its approximated hermitian $\mathscr{L}_0(E)$ by an exponentially small correction. From this, we deduce that if $\det_0(E_{0,\mathrm{res}})=0$ for $E_{0,\mathrm{res}}$ on the real axis, then $\det(E_{0,\mathrm{res}}+\delta E_{\mathrm{res}})=0$ for an exponentially small $\delta E_{\mathrm{res}}$. As we have seen before, because $\mathscr{L}(E)$ arises from an hermitian problem after tracing out the reservoirs, we know that $\Im\,\delta E_{\mathrm{res}}<0$.

### Appendix B: Spectral decomposition for current operators

The particle current operator from the dot to reservoir $j$ reads, in Schrödinger's picture:

$$\hat{I}_i(t)=-iJ_i\sum_\sigma\left(e^{-is_i\omega_0 t}\Psi^\dagger_\sigma(i)d_\sigma-e^{is_i\omega_0 t}d^\dagger_\sigma\Psi_\sigma(i)\right),,\qquad\text{(B1)}$$

where

$$\Psi^\dagger_\sigma(i)=\int\frac{d^D\mathbf{k}}{(2\pi)^D}c^\dagger_\sigma(i,\mathbf{k})\qquad\text{(B2)}$$

is the electron creation operator at the point in reservoir $i$, which is facing the dot across the tunnel barrier. To compute correlation functions involving current operators, the first step is to give a spectral decomposition of Heisenberg operators $\Psi^\dagger_\sigma(i,t)$ in terms of dressed quasi-particle operators $\Gamma^\dagger_\sigma(j,\mathbf{k})$ and $\Gamma_{-\sigma}(j,\mathbf{k})$. Such decomposition is similar to the one for dot operators, see Eq. (15) above, and it reads

$$\begin{aligned}e^{-is_i\omega_0 t}\Psi^\dagger_\sigma(i,t)=&\sum_{j=1}^N J_i\int\frac{d^D\mathbf{k}}{(2\pi)^D}\sum_{m\in\mathbb{Z}}e^{i(E(j,\mathbf{k})+m\omega_0)t}\bar{U}^{(i)}_m(j,\mathbf{k})\Gamma^\dagger_\sigma(j,\mathbf{k})\\&+\sum_{j=1}^N J_i\int\frac{d^D\mathbf{k}}{(2\pi)^D}\sum_{m\in\mathbb{Z}}\sigma e^{-i(E(j,\mathbf{k})+m\omega_0)t}V^{(i)}_m(j,\mathbf{k})\Gamma_{-\sigma}(j,\mathbf{k})\qquad\text{(B3)}\\&+\int\frac{d^D\mathbf{k}}{(2\pi)^D}\left(\bar{x}(i,\mathbf{k})e^{-i\varphi_i/2}e^{i(E(i,\mathbf{k})-s_i\omega_0)t}\Gamma^\dagger_\sigma(i,\mathbf{k})-\sigma y(i,\mathbf{k})e^{-i\varphi_i/2}e^{-i(E(i,\mathbf{k})+s_i\omega_0)t}\Gamma_{-\sigma}(i,\mathbf{k})\right),\end{aligned}$$

where $U^{(i)}_m(j,\mathbf{k})$ and $V^{(i)}_m(j,\mathbf{k})$ have been defined in Eqs. (10) and (11). We note that the first two terms in Eq. (B4) are linear in the resolvent through $U^{(i)}_m(j,\mathbf{k})$ and $V^{(i)}_m(j,\mathbf{k})$, whereas the last term does not involve the resolvent. For various purposes, such as checking current conservation, it is useful to transform this last term using Eqs. (8) and (9). This gives

$$\begin{aligned}J_ie^{-is_i\omega_0 t}\Psi^\dagger_\sigma(i,t)=&\int\frac{d^D\mathbf{k}}{(2\pi)^D}\sum_{m\in\mathbb{Z}}e^{im\omega_0 t}\sum_{j=1}^N\left(J_i^2\bar{U}^{(i)}_m(j,\mathbf{k})e^{iE(j,\mathbf{k})t}\Gamma^\dagger_\sigma(j,\mathbf{k})-J_j^2\bar{U}^{(j)}_m(i,\mathbf{k})e^{iE(i,\mathbf{k})t}\Gamma^\dagger_\sigma(i,\mathbf{k})\right)\qquad\text{(B4)}\\&+\sigma\int\frac{d^D\mathbf{k}}{(2\pi)^D}\sum_{m\in\mathbb{Z}}e^{-im\omega_0 t}\sum_{j=1}^N\left(J_i^2V^{(i)}_m(j,\mathbf{k})e^{-iE(j,\mathbf{k})t}\Gamma_{-\sigma}(j,\mathbf{k})-J_j^2V^{(j)}_m(i,\mathbf{k})e^{-iE(i,\mathbf{k})t}\Gamma_{-\sigma}(i,\mathbf{k})\right)\\&+\int\frac{d^D\mathbf{k}}{(2\pi)^D}\sum_{m\in\mathbb{Z}}(E(i,\mathbf{k})+m\omega_0)\left(\bar{u}_m(i,\mathbf{k})e^{i(E(i,\mathbf{k})+m\omega_0)t}\Gamma^\dagger_\sigma(i,\mathbf{k})+\sigma v_m(i,\mathbf{k})e^{-i(E(i,\mathbf{k})+m\omega_0)t}\Gamma_{-\sigma}(i,\mathbf{k})\right).\end{aligned}$$

Inserting this spectral decomposition and the one already given for operators on the dot in the above definition of the current operator $\hat{I}_i(t)$ shows that we can write

$$\sum_\sigma\langle S|\hat{I}_{i,H}(t)|S\rangle=\sum_{p\in2\mathbb{Z}}B_{i,p}e^{-ip\omega_0 t},\qquad\text{(B5)}$$

with

$$B_{i,p} = 2i\sum_{j=1}^{N}\int\frac{d^D\mathbf{k}}{(2\pi)^D}\left(\sum_{m\in\mathbb{Z}}^{(j)} J_i^2 V_m^{(i)}(j,\mathbf{k})\bar{v}_{m-p}(j,\mathbf{k}) - \sum_{m\in\mathbb{Z}}^{(i)} J_j^2 V_m^{(j)}(i,\mathbf{k})\bar{v}_{m-p}(i,\mathbf{k})\right)$$
$$+\,\text{c.c.}\;(p\to -p) + 2ip\omega_0\int\frac{d^D\mathbf{k}}{(2\pi)^D}\sum_{m\in\mathbb{Z}}^{(i)} v_m(i,\mathbf{k})\bar{v}_{m-p}(i,\mathbf{k}). \tag{B6}$$

As often in this paper, an $(i)$ superscript over the summation over $m$ means that $m$ is required to have the same parity as $s_i$.

We can now use the narrow resonance approximation, as in subsection II, which gives

$$B_{i,p} = 2i\sum_{j=1}^{N}\sum_{\alpha=\pm} S_{j,\alpha}\sum_{m\in\mathbb{Z}}^{(j)} J_i^2\left(g^{(i)}\Psi\right)_{m,v}\bar{\Psi}_{m-p,v}(E_\alpha) - 2i\sum_{j=1}^{N}\sum_{\alpha=\pm} S_{i,\alpha}\sum_{m\in\mathbb{Z}}^{(i)} J_j^2\left(g^{(j)}\Psi\right)_{m,v}\bar{\Psi}_{m-p,v}(E_\alpha)$$
$$+\,\text{c.c.}\;(p\to -p) + 2ip\omega_0\sum_{\alpha=\pm} S_{i,\alpha}\sum_{m\in\mathbb{Z}}^{(i)} \Psi_{m,v}(E_\alpha)\bar{\Psi}_{m-p,v}(E_\alpha). \tag{B7}$$

Here, we have defined

$$\left(g^{(i)}\Psi\right)_{m,v}(E_\alpha) = -g_{21}^{(i)}(E_\alpha + (m-s_i)\omega_0)\Psi_{m-2s_i,u}(E_\alpha) + g_{22}^{(i)}(E_\alpha + (m-s_i)\omega_0)\Psi_{m,v}(E_\alpha). \tag{B8}$$
